# Supplementary material for: A hybrid Green-Kubo (hGK) framework for calculating viscosity from short MD simulations
Source: arXiv:2512.04546 source file (2026-03-12)
Supplement: Supplementary file 1 [file hybridGK_viscosity_si.pdf]

*Supplementary Information for*  
**A hybrid Green-Kubo (hGK) framework for calculating viscosity from short MD simulations**

Akash K. Meel<sup>a,\*</sup> and Santosh Mogurampelly<sup>a,b,\*</sup>

<sup>a</sup>Polymer Electrolytes and Materials Group (PEMG), Department of Physics, Indian Institute of Technology Jodhpur, Karwar, Rajasthan 342030, India

<sup>b</sup>Currently on a sabbatical at the Department of Physics, College of Science, Sultan Qaboos University, Al Khod 123, Oman

**Contents of the SI:** The supplementary information contains: (**Section S1**) Applying the hGK approach to liquid Ar. (**Section S2**) Calculation of the computational time speedup and the speedup values for the various systems studied in this work.

\*Authors to whom correspondence should be addressed: [akmeel.3600@gmail.com](mailto:akmeel.3600@gmail.com), and [santosh@iitj.ac.in](mailto:santosh@iitj.ac.in)

### Section S1. Applying the hGK approach to liquid Ar.

Liquid argon serves as a simple reference system for validating tail-continuation schemes due to its minimal structural complexity and short relaxation times. The simulation protocol follows that used for the water and electrolyte systems in the main text. Argon atoms interact through a Lennard-Jones potential that produces a single monotonic decay of the stress autocorrelation function. The absence of bonded interactions eliminates the slow collective relaxations that appear in molecular and polymeric liquids. As a result, the decay of the SACF is fully described by a single relaxation mode with no secondary tail.

The hybrid method is applied using the same procedure described in the main paper. Argon was modeled using Lennard-Jones parameters ( $\sigma$  and  $\epsilon$ ) reported by White et al.<sup>1</sup> The lower cutoff time  $\tau_l$  is identified at the end of the short vibrational decay, and the upper cutoff  $\tau_u$  is varied until the predicted viscosity converges. The stretched exponential form provides a stable continuation even for this simple system, although the exponential and stretched exponential models yield nearly identical viscosities due to the narrow relaxation spectrum. The hGK predicted viscosity agrees closely with the results obtained from traditional GK within statistical error, which confirms that the hGK approach remains accurate when applied to simple liquids that lack slow relaxation dynamics.

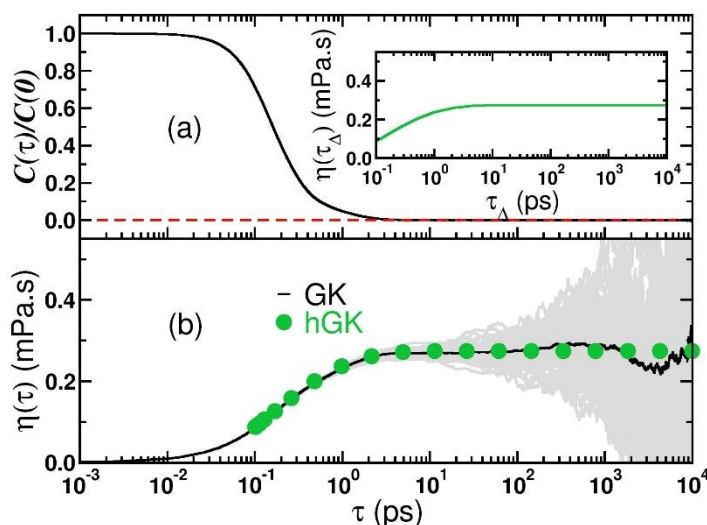

**Fig. S1:** Demonstration of hGK framework for liquid Ar: **(a)** Normalized SACF, with inset showing the dependence of predicted viscosity on the window size. **(b)** Running integral of SACF

with the black solid line representing data from the traditional GK framework, and the green circles represent the appended values using the hybrid approach. The hGK framework and the GK agree well.

## **Section S2. *Calculating computational time speedup***

In addition to improving numerical stability, the hGK framework provides a significant computational acceleration. The primary source of savings arises from the SACF evaluation itself. Traditional approaches to calculating correlation functions, which use brute force multiplication, scale as  $O(N^2)$  operations for a trajectory of  $N_{\text{frames}}$  number of data points.<sup>2,3</sup> By contrast, applying the Wiener-Khinchin theorem reduces the operation count to  $O(N\log_2 N)$  by computing the SACF through the power spectrum of the stress-tensor time series.<sup>4,5</sup> Using the FFT approach to calculate the SACF provides a substantial speedup for both the GK and hGK frameworks.

Generating this input data for both GK and hGK requires equilibrium MD simulations of multiple independent trajectories, and this is a major contribution to the total computational cost. The additional speedup offered by the hGK framework arises because it allows the use of shorter trajectories. To accurately predict the shear viscosity using hGK, one only needs to resolve the SACF up to a chosen upper cutoff  $\tau_u$ . For longer lag times, the SACF is calculated analytically using the chosen tail model. As a result, the time evolution of the pressure tensor does not need to be sampled over the full time span required by the GK framework; instead, it suffices to gather high-quality statistics only up to  $\tau_u$ . The total time to compute the viscosity can therefore be written as  $t_\eta = t_{\text{MD}} + t_{\text{SACF}}$ , where  $t_{\text{MD}}$  is the time needed to perform the MD simulations and generate the stress-tensor time series for all  $N_{\text{traj}}$  independent runs, and  $t_{\text{SACF}}$  is the time needed to evaluate the SACF from those trajectories using the FFT-based Wiener–Khinchin procedure. The traditional GK framework requires  $N_{\text{frames}}$  time points to resolve the full relaxation of the SACF. In the hGK framework, we only need shorter trajectories of length  $N'$ , such that  $N_{\text{frames}} = \alpha N'$ .

In practice,  $N'$  is chosen so that the time window up to  $\tau_u$  is sampled with good statistics; as a rule of thumb, one may take  $N' \approx 10\tau_u$ . With this notation, the computational cost of the hGK method can be written as

$$t_\eta^{\text{hGK}} \approx xN' + N'\log N',$$

where  $x$  is the effective time per frame required to simulate  $N_{\text{traj}}$  independent trajectories. The first term represents the MD cost to generate trajectories of length  $N'$ ; the second term represents the FFT-based SACF evaluation over those  $N'$  frames. Similarly, for the GK framework, we can write

$$t_{\eta}^{\text{GK}} \approx xN_{\text{frames}} + N_{\text{frames}} \log N_{\text{frames}} = x\alpha N' + \alpha N' \log (\alpha N').$$

The overall speedup factor is then

$$S = \frac{t_{\eta}^{\text{GK}}}{t_{\eta}^{\text{hGK}}} = \frac{x\alpha N' + \alpha N' \log (\alpha N')}{xN' + N' \log N'} = \alpha \frac{x + \log (\alpha N')}{x + \log N'}.$$

When SACF calculation is very efficient and the MD cost dominates, the logarithmic contributions become negligible compared to  $x$ . In this limit, the expression simplifies to  $S \approx \alpha$ , so the hGK approach yields a speedup that scales as  $O(\alpha)$  in the total wall-clock time for viscosity estimation. If we are interested in isolating only the speedup in the SACF evaluation, ignoring MD costs, then

$$S_{\text{SACF}} = \frac{N_{\text{frames}} \log N_{\text{frames}}}{N' \log N'} = \frac{\alpha N' \log (\alpha N')}{N' \log N'} = \alpha \frac{\log (\alpha N')}{\log N'}.$$

Thus, for the SACF calculations alone, the speedup scales as  $S_{\text{SACF}} = O(\alpha \frac{\log (\alpha N')}{\log N'})$ , with the leading gain again controlled by the factor  $\alpha$  that quantifies the reduction in the number of frames.

| System     | $N_{\text{frames}}$ | $N'$   | $\alpha$ | $S$    |
|------------|---------------------|--------|----------|--------|
| Liquid Ar  | $10^5$              | $10^3$ | $10^2$   | $10^2$ |
| Water      | $10^5$              | $10^3$ | $10^2$   | $10^2$ |
| EC-LiTFSI  | $10^7$              | $10^4$ | $10^3$   | $10^3$ |
| PEO-LiTFSI | $10^9$              | $10^6$ | $10^3$   | $10^3$ |

**Table S1:** Summary of the computational speedup  $S$  for the different systems considered in this work. Here  $N$  represents the number of frames required to accurately sample the stress tensor to obtain a plateau in the running integral of the SACF, and  $N'$  represents the number of frames required by the hGK approach proposed in this work.

## References:

- (1) White, J. A. Lennard-Jones as a Model for Argon and Test of Extended Renormalization Group Calculations. *J Chem Phys* 1999, *111* (20), 9352–9356. <https://doi.org/10.1063/1.479848>.
- (2) Frenkel, Daan.; Smit, Berend. *Understanding Molecular Simulation : From Algorithms to Applications*; Academic Press, 1996.
- (3) Allen, M. P.; Tildesley, D. J. *Computer Simulation of Liquids*; Oxford University Press, 2017. <https://doi.org/10.1093/oso/9780198803195.001.0001>.
- (4) Wiener, N. Generalized Harmonic Analysis. *Acta Mathematica* 1930, *55* (0), 117–258. <https://doi.org/10.1007/BF02546511>.
- (5) Khintchine, A. Korrelationstheorie Der Stationären Stochastischen Prozesse. *Math Ann* 1934, *109* (1), 604–615. <https://doi.org/10.1007/BF01449156>.
